# Supplementary material for: AGPNet -- Autonomous Grading Policy Network
Source: arXiv:2112.10877 source file (2021-12-20)
Supplement: Supplementary file 1 [file appendix.tex]

\section{Appendix}\label{Appendix}

\section{Algorithm Details} \label{app:training_details}
Here we give a deeper explanation for each training algorithm.
\subsection{Behaviour Cloning - BC}

\paragraph{Algorithm}
In BC, we train the policy network \newline $\pi_\theta=P(p_t)*P(s_t)$ in a supervised learning manner where we minimize the distance from way-points selected by the behaviour policy to the ones sampled from our trained policy distribution. Most BC algorithms minimize $l_1$ or $_2$ losses, but we chose to use the binary cross entropy function instead from training robustness reasons. Given the behaviour Dataset, $(S_t, a_t) \in D_B$, and the policy network prediction $a_{t_\theta} \sim \pi_\theta(a_t|S_t)$:
$$L_{BC}(\theta) = \mathbb{L}_{CE}(\pi_\theta(a_{t_\theta}),\pi_B(a_{t_B}))$$
where $\mathbb{L}_{CE}(\cdot)$ is the binary cross-entropy loss.

\paragraph{Training}

During training, the dataset included $150$ episodes each with a ranging number of states.
In Figure \ref{fig:bc_loss} we see the evaluation loss over time. Both BC and BC+CL converge withing $250$ steps. 
% In Figure \ref{fig:bc_training_example} an example of our training results can be viewed where the the inputs to the model are on the left and the action distributions in the middle (for action $p$) and right (for action $s$). 
% Figure \ref{fig:bc_dist_rand} shows the probabilities before training where the Gaussian layer is clearly viewed,
% whereas \ref{fig:bc_dist_gaus} shows the results after $10$ epochs, showing the start of conversion to a single deterministic policy.  

In PPO the loss can be divided into two parts:
$$L_A = \frac{\pi_{\theta}(a|s)}{\pi_{\theta_k}(a|s)}  A^{\pi_{\theta_k}}(s,a)$$  
$$L_B = {clip}\left(\frac{\pi_{\theta}(a|s)}{\pi_{\theta_k}(a|s)}, 1 - \epsilon, 1+\epsilon \right) A^{\pi_{\theta_k}}(s,a)$$
In addition we train the value function using supervised learning mechanisms between the value network and value calculated for a given trajectory:
$$L_V = MSE(V_\theta, V_{calc})$$
The combined loss is then:

$$L_{PPO}(s,a,\theta_k,\theta) = \min\left(L_A, L_B\right) + \lambda_v * L_V$$
where $A^{\pi_{\theta_k}}(s,a)$ is the advantage function, $L_V$ is the value function loss.

\paragraph{Training}
In Figure \ref{fig:rl_loss} we show the mean reward calculated during training on $50$ different initial episodes. As seen in the Figure, RL+BC+CL reaches the best overall reward faster than other policies. In addition, RL+CL continues to learn throughout all steps. Note that the std. shown in the Figure is large due to a variety of scenarios (each scenario can reach a different reward depending on the initial amount of sand piles).

%%%%%%%%%%%%%%%%%%%%%%%%%%%%%%%%%%%%%%%%%%%%%%%%%%%%%%%%%%%%%%
\subsection{CL implementation} \label{app:CL_implementation}
Our CL implementation was inspired by \cite{srinivas2020curl} with the following modifications: (i) additional random cropping was not done to the state space as Gaussian masking was applied to the input image and effectively cropped out relevant sections in state space without technically changing the image size.
(ii) from training stability considerations, we trained CL loss $10$ times for each training iteration. CL loss is not changed from \cite{srinivas2020curl}.
